# Supplementary material for: Optical properties and carrier localization in the layered phosphide EuCd$_\mathbf{2}$P$_\mathbf{2}$
Source: arXiv:2209.10606 source file (2023-03-21)
Supplement: Supplementary file 1 [file supplemental.pdf]

# Supplementary Material for:
# Optical properties and carrier localization in the layered phosphide $EuCd_2P_2$

C. C. Homes,[1,*] Z.-C. Wang,[2] K. Fruhling,[2] and F. Tafti[2,†]

[1] *National Synchrotron Light Source II, Brookhaven National Laboratory, Upton, New York 11973, USA*
[2] *Department of Physics, Boston College, Chestnut Hill, Massachusetts 02467, USA*

(Dated: November 10, 2022)

## I. TUTORIAL ON VIBRATIONAL LINE SHAPES

Infrared-active vibrational modes play a dominant role in the optical properties of bad metals and semiconductors due to the either poor or total absence of electronic screening [1]. The optical properties may be described by the Drude-Lorentz model for the dielectric function $\tilde{\epsilon} = \epsilon_1 + i\epsilon_2$, described in the main text but repeated here again for convenience,

$$\tilde{\epsilon}(\omega) = \epsilon_\infty - \frac{\omega_{p,D}^2}{\omega^2 + i\omega/\tau_D} + \sum_j \frac{\Omega_j^2}{\omega_j^2 - \omega^2 - i\omega\gamma_j}, \tag{S1}$$

where $\epsilon_\infty$ is the real part of the dielectric function at high frequency, $\omega_{p,D}^2 = 4\pi n e^2/m^*$ is the square of the plasma frequency with carrier concentration $n$ and effective mass $m^*$, and $1/\tau_D$ is the optical scattering rate for the delocalized (Drude) carriers. In the summation, $\omega_j$, $\gamma_j$ and $\Omega_j$ are the position, width, and strength of the $j$th vibration or bound excitation, respectively. The complex conductivity is

$$\tilde{\sigma} = \sigma_1 + i\sigma_2 = \frac{2\pi}{Z_0} i\omega \left[\epsilon_\infty - \tilde{\epsilon}(\omega)\right], \tag{S2}$$

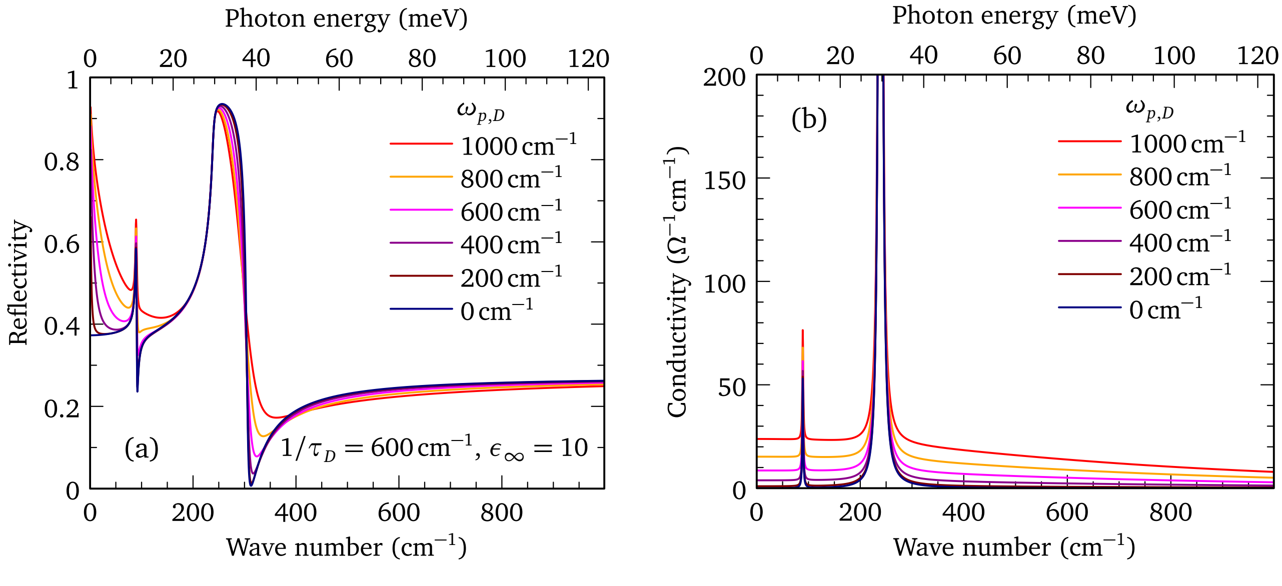


Figure S1. The calculated (a) reflectivity and (b) real part of the optical conductivity for a Drude-Lorentz model with two infrared-active modes, and free-carrier (Drude) component that gradually increases from $\omega_{p,D} = 0$ to 1000 cm$^{-1}$. The introduction of a weak electronic background has the effect of washing out the deep minima in the line shapes in the reflectivity, while in the optical conductivity the peaks associated with the infrared-active modes retain their amplitude and line shapes, and are simply superimposed upon a weak electronic background of $\sigma_1 \simeq 20\ \Omega^{-1}$cm$^{-1}$.

* homes@bnl.gov
† fazel.tafti@bc.edu

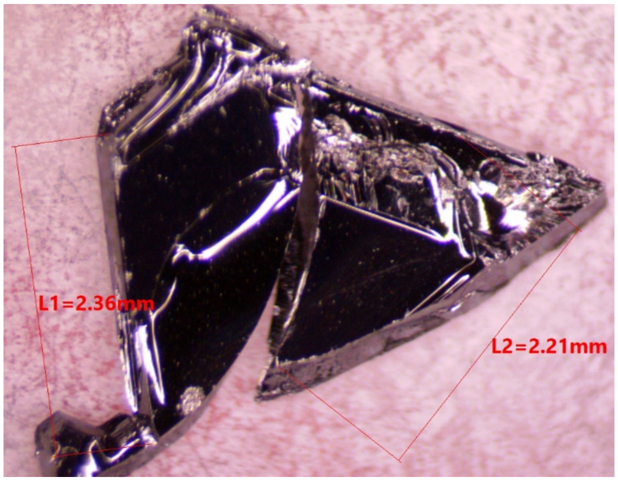


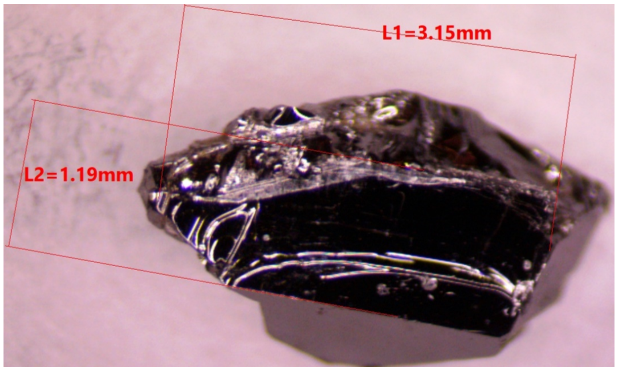


Figure S2. Single crystals of $EuCd_2P_2$ used in the reflectivity experiments. On the left-hand side is a crystal with an *ab*-plane [(001)] surface; this sample actually consists of two pieces; the piece on the left was selected for the in-plane reflectivity experiments. The sample on the right was determined to have an *a*-*c* [(101)] face. Both samples show examples of terraces on the crystals surfaces.

(in units of $\Omega^{-1}\text{cm}^{-1}$), where $Z_0 = 377\ \Omega$ is the impedance of free space. The complex refractive index is $\tilde{n} = n + ik$, where

$$n = \left[\frac{1}{2}\left(\sqrt{\epsilon_1^2 + \epsilon_2^2} + \epsilon_1\right)\right]^{1/2}, \text{ and } k = \left[\frac{1}{2}\left(\sqrt{\epsilon_1^2 + \epsilon_2^2} - \epsilon_1\right)\right]^{1/2}. \tag{S3}$$

The reflectance at a normal angle of incidence is then

$$R = \frac{(n-1)^2 + k^2}{(n+1)^2 + k^2}. \tag{S4}$$

To illustrate how even a weak electronic background can introduce large changes to the vibrational line shape in the reflectivity, we will consider two infrared-active modes of similar character to those observed in $EuCd_2P_2$ [see Figs. 4(a) and 4(b) in the main text], with $\omega_1 = 89$, $\gamma_1 = 2$, and $\Omega_1 = 80$ cm$^{-1}$, and $\omega_2 = 239$, $\gamma_2 = 5$, and $\Omega_2 = 600$ cm$^{-1}$, with $\epsilon_\infty = 10$ to reproduce the reflectivity at $\simeq 1000$ cm$^{-1}$. Initially, we consider the case of an insulator (semiconductor) in which the free carrier component is completely gapped out ($\omega_{p,D} = 0$). The resulting vibrational line shapes shown in Fig. S1(a) are extremely sharp, dispersive features; in the case of the low-frequency mode, the minima is about $R \simeq 0.22$, while for the high-frequency mode, $R \simeq 0$ at about 300 cm$^{-1}$. As the Drude component is gradually introduced, with $\omega_{p,D}$ increasing from zero to 1000 cm$^{-1}$ in 200 cm$^{-1}$ increments, with $1/\tau_D = 700$ cm$^{-1}$, the intercept on the ordinate changes immediately from $R \simeq 0.4$ to unity as soon as $\omega_{p,D} \neq 0$; in addition, the deep minima in the reflectivity associated with the vibrational modes is washed out, so that when $\omega_{p,D} = 1000$ cm$^{-1}$ it can no longer be observed in the low-frequency mode, and is almost non-existant in the high-frequency mode.

The calculated optical conductivity is shown in Fig. S1(b). For $\omega_{p,D} = 0$, the only features present are the two Lorentzian oscillators at 89 and 239 cm$^{-1}$; as non-zero values for $\omega_{p,D}$ are introduced, a Drude background (a Lorentzian centered at zero frequency with a width of $1/\tau_D$) develops. The infrared modes retain their amplitude and line shape, and are simply superimposed upon this electronic background. This is in stark contrast to the large changes observed in the vibrational line shapes in the reflectivity, illustrating how line shapes can be sensitive probes to small changes in the electronic background.

## II. TERRACING ON THE CRYSTAL FACES

Single crystals of $EuCd_2P_2$ display mirror-like as-grown surfaces, but at the same time may also have steps, or terraces, on the crystal face. This phenomena is shown in crystals in Fig. S2; the sample on the left-hand side of the figure was determined by x-ray diffraction to have an *ab*-plane [(001)] surface. This sample consisted of two pieces; the section on the left was selected for the reflectivity measurements. While the surfaces are of optical quality, there is a prominent step running through the middle of the crystal. The sample shown on the right-hand side of Fig. S2

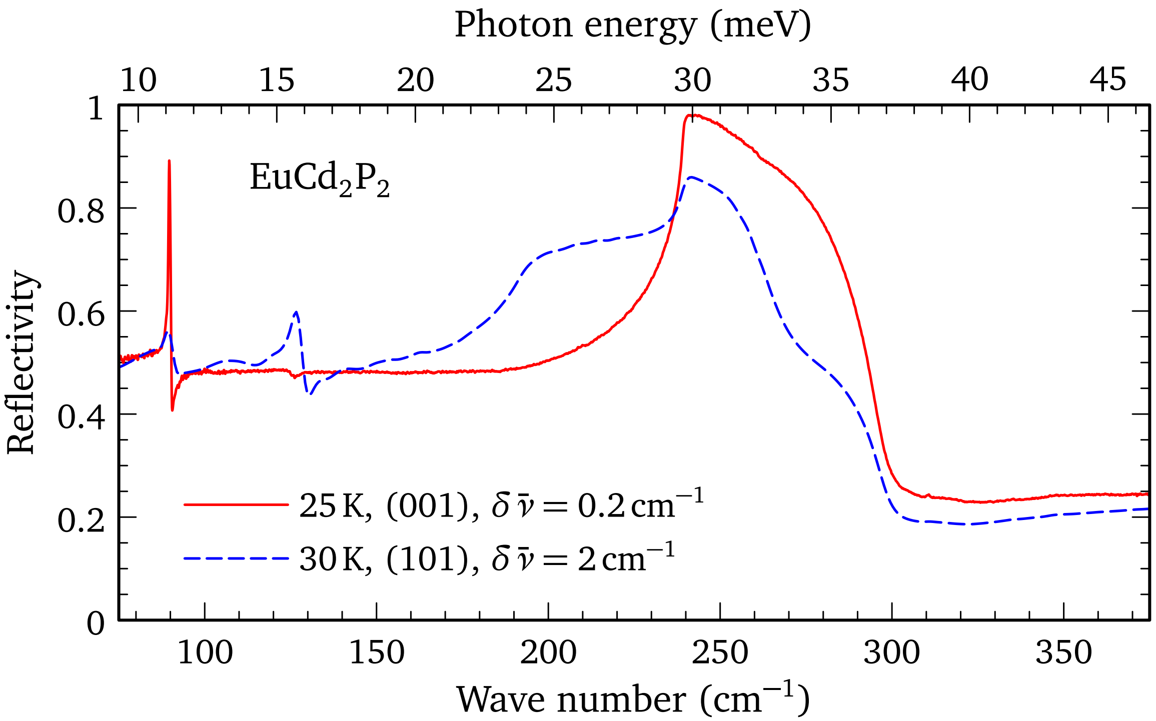


Figure S3. The reflectivity of $EuCd_2P_2$ at 25 K for light polarized in the *a*-*b* [(001)] planes with an instrumental resolution of 0.2 cm$^{-1}$ (solid line); the two features due to the $E_u$ modes are clearly observed at $\simeq$ 89 and 239 cm$^{-1}$, but in addition, there is a weak antiresonance at $\simeq$ 126 cm$^{-1}$. The reflectivity of a crystal with an *a*-*c* [(101)] face has also been measured at 30 K (dashed line) with an instrumental resolution of 2 cm$^{-1}$; in addition to the two $E_u$ modes observed in the in-plane measurements, there are two new features at $\simeq$ 126 and 206 cm$^{-1}$, associated with the $A_{2u}$ modes active along the *c* axis. Note that the low-frequency $A_{2u}$ mode corresponds precisely with the antiresonance observed in the reflectivity in the *a*-*b* plane measurement.

was determined by x-ray diffraction to have an *a*-*c* face [(101)] surface. Preliminary measurements on this crystal have been used to estimate the positions of the *c*-axis lattice modes that are further discussed in the next section.

## III. *C*-AXIS CONTRIBUTIONS TO THE *A*-*B* PLANE OPTICAL PROPERTIES

The high-resolution (0.2 cm$^{-1}$) reflectivity of $EuCd_2P_2$ is shown for light polarized in the *a*-*b* plane in Fig. S3; the two prominent infrared-active $E_u$ modes are observed at $\simeq$ 89 and 239 cm$^{-1}$. (A simple empirical valence force-field model reproduces the experimental frequencies and intensities. The in-plane atomic displacements of the low-frequency $E_u$ mode consist of the out-of-phase displacements of the Eu and Cd atoms, with only a minor contribution from the P atoms, which are in phase with the Cd atoms. The high-frequency mode consists mainly of the displacement of P atom, which is out-of-phase to the Cd and Eu atoms.) Superimposed on this result is the reflectivity of the *a*-*c* face with a slightly lower resolution (2 cm$^{-1}$) which clearly shows features associated with the $A_{2u}$ *c*-axis modes. However, the high-frequency $A_{2u}$ mode overlaps with the strong $E_u$ mode, making this reflectivity difficult to fit; it is easier to fit the optical conductivity. The optical conductivity has been determined from a Kramers-Kronig analysis [2] of the reflectivity of the sample with the *a*-*c* face at 30 K by employing a metallic extrapolation at low frequency, and by assuming a constant reflectance above the highest measured frequency point up to $5 \times 10^4$ cm$^{-1}$, above which a free-electron approximation is employed [3]. The results for the real and imaginary parts of the optical conductivity of $EuCd_2P_2$ at 30 K are shown in Figs. S4(a) and S4(b), respectively.

The model in Eq. (S1) has been fit simultaneously to the real and imaginary parts of the complex conductivity in the far-infrared region using a non-linear least-squares technique. The conductivity is described by a Drude component as well as four Lorentz oscillators. The results of the fit are shown by the dashed line in Figs.S4(a) and S4(b), respectively, and are summarized in Table I. The low-frequency $E_u$ mode is observed at 89.7 cm$^{-1}$ in the *a*-*c* face, which is almost exactly the value observed in the *a*-*b* planes, 89.4 cm$^{-1}$; the next two modes at $\simeq$ 126.6 and 201.6 cm$^{-1}$ are assigned to the *c*-axis $A_{2u}$ modes. The fit to the weak shoulder at $\simeq$ 240 cm$^{-1}$, which is the position of the high-frequency $E_u$

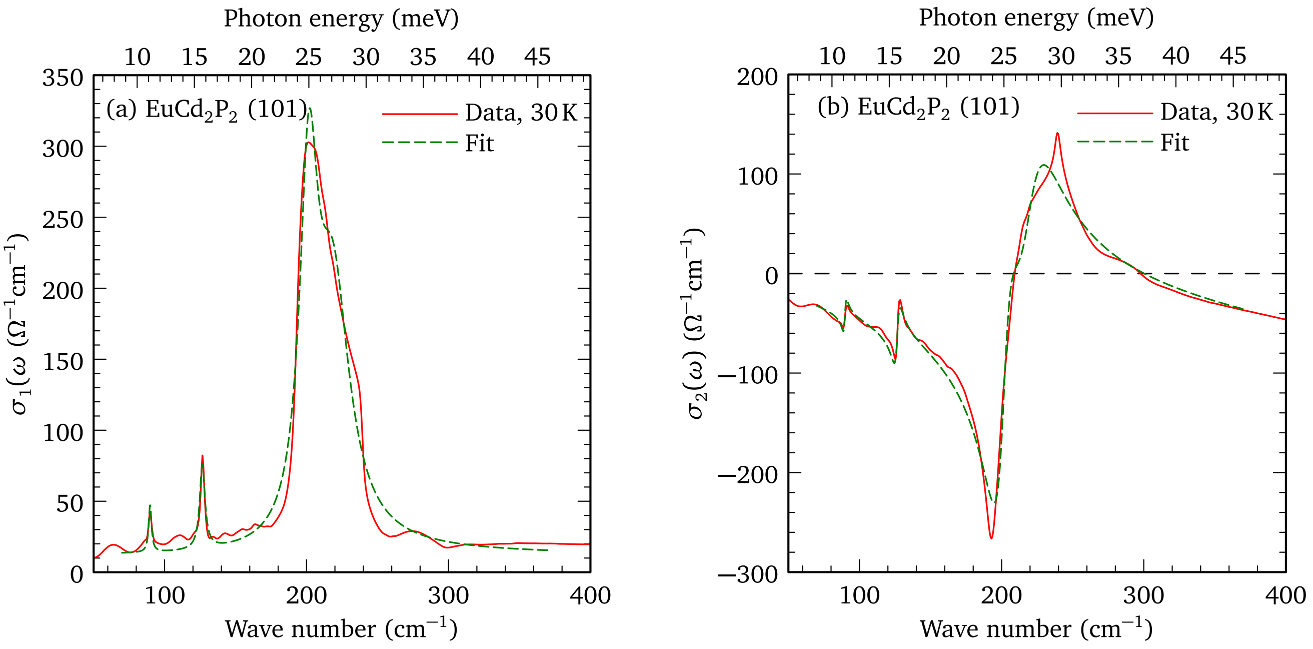


Figure S4. (a) The real part of the optical conductivity for $EuCd_2P_2$ at 30 K for light polarized in an *a*-*c* plane (solid line); the dashed line is the fit to Eq. (S1). (b) The imaginary part of the complex conductivity (solid line) and the fit (dashed line). Note that in both cases the fit to the shoulder in the real part and the peak in the imaginary part of the optical conductivity at $\simeq 240$ cm$^{-1}$ is rather poor and, where applicable, the line widths are significantly broader than those observed in the *a*-*b* plane conductivity.

mode, is rather poor; in addition, the widths of the two high-frequency modes are considerably larger than the value for the $E_u$ mode from the *a*-*b* plane measurement with a similar resolution, which suggests that the *a*-*c* face response is more complicated than the simple Drude-Lorentz model being employed here. The fit to the imaginary part of the optical conductivity allows the the high-frequency part of the dielectric function to be determined, $\epsilon_\infty \simeq 12$. Because the Kramers-Kronig analysis has been performed on a limited frequency range, there is some uncertainty attached to this value.

There are several ways that the *c*-axis optical properties may manifest themselves in the *a*-*b* plane response. The first may be a simple mixture of the *a*-*b* plane and *c* axis reflectivity. The second may arise from surface misorientations that allow the *c* axis longitudinal optic (LO) modes to appear as resonances (antiresonances) in insulating (metallic) systems [4–6]. The position of the LO mode may be estimated from the position and strength of the transverse optic (TO) mode,

$$\omega_{\rm LO}^2 \simeq \omega_{\rm TO}^2 + \frac{\Omega_0^2}{\epsilon_\infty}. \quad (S5)$$

The value for the LO mode depends heavily on the value of $\epsilon_\infty$. To ensure that the value for $\epsilon_\infty \simeq 12$ returned from the fits is reasonable, we examine the optical properties in the *a*-*b* plane, where the strong $E_u$ mode at $\simeq 239$ cm$^{-1}$ is clearly identified. The temperature dependence of this mode is shown on the left-hand side of Fig. S5 and is indicated by the label “TO”; it should be noted that on this scale the strength of the mode and its symmetric line shape are self evident. The LO mode for this vibration should manifest itself as a peak in the loss function, $-{\rm Im}[1/\tilde\epsilon(\omega)]$, shown on the right-hand side of Fig. S5 and denoted by the label “LO”; peak in the loss function occurs at $\simeq 296$ cm$^{-1}$ at $\simeq 15$ K where the background conductivity is reduced due to the more resistive nature of the sample (increasing the background conductivity has the effect of smearing out peak in the loss function). Using these values for the positions of the LO and TO modes, and using $\Omega_0 \simeq 600$ cm$^{-1}$ from Fig. 4(b), then Eq. (S5) yields $\epsilon_\infty = 11.8$, which is very close the value of 12 returned from the fit, validating the earlier result and suggesting that $\epsilon_\infty$ likely has little in the way of any asymmetry.

Using the fitted values for the TO modes in Fig. S4 and $\epsilon_\infty = 12$, the estimated values for the LO modes are listed in Table I. The fact that the antiresonance in Fig. S3 occurs at exactly the same frequency as the peak in the optical conductivity, $126.6 \pm 0.8$ cm$^{-1}$, implies that it is associated with the *c*-axis $A_{2u}$ TO mode rather than the LO mode, estimated to be occur at $\simeq 131.7$ cm$^{-1}$ indicating that the *c*-axis contamination arises simply from the mixing of the *a*-*b* plane and *c* axis reflectivities due to the presence of *c*-axis steps, or terraces, in the *a*-*b* plane face.

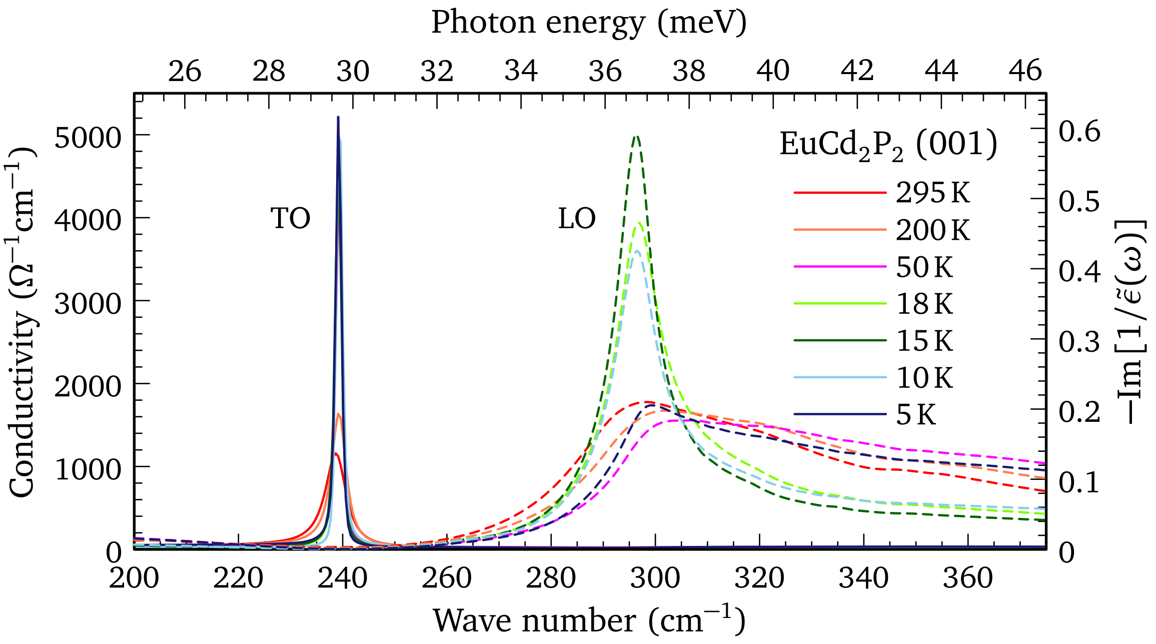


Figure S5. The temperature dependence of the optical conductivity (solid lines, left axis) and the loss function (dashed lines, right axis) for the strong $E_u$ mode in $EuCd_2P_2$ for light polarized in the *a*-*b* [(001)] plane. The TO mode is very strong and narrow, with the maximum observed at $\simeq 239$ cm$^{-1}$, while the LO mode is broader with a maximum of $\simeq 296$ cm$^{-1}$ at about 15 K where the resistivity in the sample is close to its maximum (increasing the electronic background has the effect of smearing out the loss function in the region of the LO mode).

Table I. The parameters for the Drude-Lorentz model fitted to the real and imaginary parts of the optical conductivity $EuCd_2P_2$ at 30 K light polarized in an *a*-*c* plane. The Drude values are $\omega_{p,D} \simeq 1468$ cm$^{-1}$ and $1/\tau_D \simeq 1070$ cm$^{-1}$. All values are in units of cm$^{-1}$, unless otherwise indicated.[a]

| Mode | $\omega_{\mathrm{TO},j}$ | $\omega_{\mathrm{LO},j}$ | $\gamma_j$ | $\Omega_j$ |
|---|---|---|---|---|
| $E_u$ | 89.7 | 91.9 | 2.4 | 69 |
| $A_{2u}$ | 126.6 | 131.7 | 4.5 | 126 |
| $A_{2u}$ | 201.6 | 245.2 | 15.8 | 484 |
| $E_u$ | 218.9 | 269.7 | 28.1 | 541 |

[a] $\epsilon_\infty = 12$.

[1] C. C. Homes, A. W. McConnell, B. P. Clayman, D. A. Bonn, R. Liang, W. N. Hardy, M. Inoue, H. Negishi, P. Fournier, and R. L. Greene, Phonon Screening in High-Temperature Superconductors, Phys. Rev. Lett. **84**, 5391 (2000).
[2] M. Dressel and G. Grüner, *Electrodynamics of Solids* (Cambridge University Press, Cambridge, 2001).
[3] F. Wooten, *Optical Properties of Solids* (Academic Press, New York, 1972) pp. 244–250.
[4] D. W. Berreman, Resonant Reflectance Anomalies: Effect of Shapes of Surface Irregularities, Phys. Rev. B **1**, 381 (1970).
[5] M. Reedyk and T. Timusk, Evidence for *a*-*b*-plane coupling to longitudinal *c*-axis phonons in high-$T_c$ superconductors, Phys. Rev. Lett. **69**, 2705 (1992).
[6] C. C. Homes, J. M. Tranquada, and D. J. Buttrey, Stripe order and vibrational properties of $La_2NiO_{4+\delta}$ for $\delta = 2/15$: Measurements and *ab initio* calculations, Phys. Rev. B **75**, 045128 (2007).
